# Supplementary material for: Leveraging Natural Language Processing to Augment Structured Social Determinants of Health Data in the Electronic Health Record
Source: arXiv:2212.07538 source file (2023-04-14)
Supplement: Supplementary file 1 [file literature_brainstorm.tex]

\documentclass{article}

\usepackage{geometry}
\geometry{letterpaper, portrait, margin=0.5in}

\usepackage[breaklinks]{hyperref}
\usepackage{url}

\usepackage[numbers, sort&compress]{natbib}

\bibliographystyle{unsrtnat}

\begin{document}

\section{To Review}

\section{SDOH in clinical text and NLP}

\citet{hatef2019assessing} - \textbf{[CITE, Helpful for all authors to read.]} Explores problems of SDOH information in a large clinical data set, including structured data and unstructured text. SDOH are identified using rule-based approaches (linguistic patterns). Extraction of SDOH from text focuses on social connection, housing, and financial strain. Paper also include some analysis of structured representation of alcohol and tobacco use.\textbf{ Need to differentiate our work from this: 1) we use state-of-the-art deep learning model, and set a pattern matching, 2)?.} Need to carefully consider our work within the prior work in this space (see Discussion section).

\citet{patra2021extracting} - \textbf{[CITE]} Review of SDOH work related to NLP. Good overview, including description of methodologies (lexicon, rule-based, supervised learning, etc.) Also includes overview of types of SDOH explored.

\citet{han2022classifying} - \textbf{[CITE]} Created a annotated data set where 13 SDOH were annotated at the sentence-level as binary indicators. Explored rule-based approaches (e.g. cTAKES), discrete approaches (LRM RF), and deep learning approaches (CNN, LSTM, and BERT). SDOH predicted as text classification task, where each SDOH is a binary label (present versus absent). BERT performed the best of all methods. Experimentation included 8 of the 13 SDOH categories.

\citet{reeves2021adaptation} - [CITE] - Introduces Moonstone, which is a rule-based NLP system for extracting social risk factors from clinical text. Moonstone utilizes term expansion that is based on semantic typing.

\citet{lowery2022using} - \textbf{[maybe CITE]} Explores the relationship between EMS transportation and SDOH using univariate and multivariate analyses. SDOH identified (extracted) using regular expressions. Describes detailed preprocessing (acronym expansion, spelling correction, lemmatization, etc.). Does not appear to present the performance of the regular expressions used.

\citet{hatef2021pilot} - \textbf{[OMIT, just abstract]}

\citet{rouillard2022evaluation} - \textbf{ [optional CITE]} Rules-based approach for extracting SDOH information. Did not read thoroughly; however, probably can omit.

\section{SDOH data and EHR}

\citet{navathe2018hospital} - \textbf{[CITE]} Explores the prevalence of social factors in structured data and physician notes. The inclusion of text-encoded social factor information increased the prevalence of the social factors four tobacco use, alcohol abuse, drug abuse, depression, housing instability, fall risk, and poor social support.

\citet{chen2020social} - \textbf{[CITE]} Review paper exploring SDOH data in the EHR and its impact on analysis and risk prediction. Work reviewing the introduction, which describes the conversion to electronic records and opportunity to enhance care delivery. Summarizes utility/usefulness of SDOH data. Does not appear to differentiate structured versus text SDOH data.

\citet{hatef2019public} - \textbf{[probably OMIT]} Relationship between patient SDOH and larger population-level community health record

\citet{wark2021engaging} - \textbf{[probably OMIT]} Focused on engaging stakeholders in the integration of SDOH information into the EHR. Relevant to Andrea and Serena's work.

\citet{cantor2018integrating} - \textbf{[probably OMIT]} Focused on the integration of SDOH information into the EHR. More policy and structure focused.

\section{Clinical text and NLP}
\citet{demner2009can} - \textbf{[probably OMIT]} Broader description of how NLP can augment clinical decision-support systems. Includes review of NLP systems and history.

\section{EHR mining more broadly}
\citet{jensen2012mining} - \textbf{[probably OMIT]} High-level survey describing the mining of EHR records, including clinical text (see page 398). Good overview of EHR data and relevant machine learning. Very high-level and probably not explicitly relevant to the SDOH paper. Includes citation regarding the heterogeneity of clinical text in ref 22 Meystre 2008.

\bibliography{mybib}

\end{document}
