# Supplementary material for: Leveraging Natural Language Processing to Augment Structured Social Determinants of Health Data in the Electronic Health Record
Source: arXiv:2212.07538 source file (2023-04-14)
Supplement: Supplementary file 4 [file cover_letter.tex]

Kevin Lybarger
Assistant Professor
Department of Information Sciences and Technology
George Mason University
4400 University Dr. MSN 1G8
Fairfax, VA 22030
klybarge@gmu.edu 


November 22, 2022 


Dr. Suzanne Bakken
Editor-in-Chief
Journal of the American Medical Informatics Association


Dear Dr. Bakken,

I am pleased to submit an original research article entitled "Leveraging Natural Language Processing to Augment Structured Social Determinants of Health Data in the Electronic Health Record" to be considered for publication in the Journal of the American Medical Informatics Association Focus Issue on Social Determinants of Health (SDOH) Extraction.

This manuscript explores the prevalence of key SDOH information within clinical notes, relative to the available SDOH information in structured data, to quantify the SDOH information gain achievable by leveraging the clinical narrative. We introduce a high-performing deep learning information extraction model for generating structured semantic representations of SDOH from the clinical narrative. We applied the SDOH extraction model to a large data set from the University of Washington with more than 200,000 patients and compared the information available through structured data and text extraction. The results demonstrate that the clinical narrative is extremely important in identifying SDOH risk factors, including tobacco use, drug use, and housing instability. This work advances SDOH information extraction and contributes to our understanding of SDOH information within the electronic health record. 

This manuscript has not been previously published and is not under consideration elsewhere. Dr. Özlem Uzuner, Dr Meliha Yetisgen, and I are co-editors on the JAMIA SDOH focus issue. We have no additional conflicts of interest to disclose. Thank you for your consideration.

Sincerely,

Kevin Lybarger
