# Supplementary material for: Leveraging Natural Language Processing to Augment Structured Social Determinants of Health Data in the Electronic Health Record
Source: arXiv:2212.07538 source file (2023-04-14)
Supplement: Supplementary file 5 [file response_document1.tex]

\documentclass[review, sort&compress]{elsarticle}

%\usepackage[letterpaper, portrait,  rmargin=2.0in]{geometry}
\usepackage[letterpaper, portrait, margin=1.0in]{geometry}
\usepackage{booktabs}

\usepackage[color=yellow,textwidth=1.5in,textsize=small]{todonotes}
\usepackage{xcolor}
\usepackage{hyperref}
\usepackage{soul}
%http://latexcolor.com/
\definecolor{comment_color}{rgb}{0.0, 0.18, 0.65}
\definecolor{internal_color}{rgb}{0.79, 0.0, 0.09}


\bibliographystyle{bst/elsarticle-num-names}
\AtBeginDocument{\colorlet{default_color}{.}}



%\color{comment_color}
%\color{default_color}  


\begin{document}

\noindent
{\huge Reviewer Response Document \par}
\bigskip

We carefully read the reviewer comments and have edited the manuscript to address as many points as possible. We interleaved our responses with the reviewers’ comments below, to provide context for the responses. A version of the manuscript indicating the associated changes is provided with the revised manuscript.

\section*{Reviewer: 1}

Comments to the Author
Thank you JAMIA editor for the opportunity to review this study.  This work aimed to assess the SDOH information gain achievable by extracting structured semantic representations of SDOH from the clinical narrative and combining these extracted representations with available structured data. The article's strengths include logical writing and the application of solid and fairly standard NLP methods. With that, the innovation of the article is not fully flashed out.

\color{comment_color}

\textbf{RESPONSE:}  To make the innovative aspects of this work more clear, we have added a Contributions subsection to the Background and Significance section and expanded the discussion of related works. Under Contributions, we discuss the novelty of using a deep learning SDOH event extractor, whereas prior deep learning SDOH work has utilized simpler SDOH representations (sentence-level labels or entities) and/or rule-based extraction approaches. We also discuss the second key innovative aspect of our work, regarding the patient population and size of the EHR data set. Prior studies have focused either on comparatively small subsets of patients (often specific disease groups) or done so using rule-based architectures alone. In contrast, we apply our deep learning extractor to an entire hospital system patient population for a calendar year. Finally, our work compares SDOH findings by NLP to that of structured data, for a much larger patient cohorts that prior work. \\

\color{default_color} 


In addition, English language needs to be revised throughout the manuscript as this study uses uncommon language, for example, “Several works treated the extraction of SDOH…”  “Works” cannot treat extraction- this is supposed to be studies or researchers.

\color{comment_color}
\textbf{RESPONSE:}  We carefully reviewed and edited the manuscript, including rephrasing the above example as "Several \textit{studies} treated the extraction...". \\

\color{default_color} 

My specific comments are provided below:  
Introduction: this section has the study description and results. This is not typical for JMIA submissions- you don’t need to present this information twice – just focus on the introduction about SDOH.

\color{comment_color}

\textbf{RESPONSE:} As suggested, we have removed the study description and results summary from the Introduction. \\

\color{default_color} 

Discussion section: This section needs to be significantly expanded. First, you need to compare your results on the frequency of NLP-derived SDOH with other studies. For example, Navathne 2016 study cited here found that using NLP, you can find `50\% of smokers. Your study only shows 19\% added people. Other studies have alos higher numbers, I believe, and this should be discussed.

\color{comment_color}
\textbf{RESPONSE:} To better contextualize our findings, we've added the following text to the Discussion: 
\begin{quote}
    ``The SDOH from our case study that can be most readily compared to prior work is that of tobacco use. 19\% of potential smokers we identified were found only by NLP, and Navarthe et al. similarly identified 15\% of patients, though only among cardiovascular disease patients and as compared to ICD-9 codes for smoking.\cite{navathe2018hospital} Yu et al.'s study of cancer cohorts similarly found 18\% of smoking information using only NLP.\cite{yu2021study} Our findings differed from Wang et al.'s, who found 52\% of a small cohort with smoking habits using NLP, but all of whom also had corresponding structured data.\cite{wang2016investigating} We hypothesize that this may be due to differing institutional practices or other confounding factors.  ''
\end{quote}


As best we can tell, the Navathe paper found an additional 15\% of smoking patients using NLP, with the remainder identified by ICD-9 codes, for 30\% total. We were unable to find a reference to 50\%, though please let us know if we are misunderstanding. The other studies discussed above found similar proportions of patients based on our review. Each of the studies mentioned used different cohort sizes, extraction architectures, and granularities of information, which limits comparability. \\

\color{default_color} 

In addition, the contribution of you innovative NLP method needs to be described. Is your method better compared to he described studies? As you suggest, there were multiple studies of SDOH extraction with NLP in the past, so how does your method advance the science and practice of SDOh extraction? Is it more efficient? Faster?  More accurate? This is key since JAMIA often accepts manuscripts with significant methods innovation- and currently, I am not sure why this study is innovative in terms of methods. 

\color{comment_color}
\textbf{RESPONSE:}  Regarding our extractor, the SHAC annotation scheme does not conform to a typical relation extraction or event extraction task, in that it includes normalized representations of key phenomena (e.g. \textit{Status Time} for \textit{Alcohol} ). Consequently, extraction of the SHAC phenomena requires adaptation of existing methods. SHAC was used in the 2022 National NLP Clinical Challenge on Extracting Social Determinants of Health Challenge (n2c2/UW SDOH Challenge).\cite{lybarger2023n2c2} Our mSpERT SDOH extractor was not developed within the scope of the n2c2/UW SDOH Challenge and differs from the shared task systems in various aspects; however, the training and evaluation data used to develop the mSpERT SDOH extractor was consistent with Subtask C of the n2c2/UW SDOH Challenge. If compared to shared task systems, the mSpERT performance would only be outperformed by two teams. We updated the Results section to include a brief description of the challenge and the performance of mSpERT, to provide context for the presented mSpERT performance results. \\

\color{default_color} 

Additional comments:
-Please provide more detail around the strengths of BERT based approaches compared to the other examples listed in Background and Significance

\color{comment_color}
\textbf{RESPONSE:} We added a brief description of pre-trained language models, including BERT, and their success within SDOH information extraction tasks. \\

\color{default_color} 

-There seems to be a lot of detail in the introduction and background/significance; however, I am not sure it is all needed. Maybe consider moving some of the other examples to the discussion to flush out why the model developed in this manuscript stands out among other approaches.

\color{comment_color}
\textbf{RESPONSE:} We've edited the Introduction to remove paper summary information that is presented in the Abstract. Additionally, we pared down the content in the Background and Significance section. \\


\color{default_color} 

- I recommend including that this study is limited by the social determinants of healths outlined by SHAC’s and misses other important social determinants (e.g., living environment, access to care, food insecurity)

\color{comment_color}
\textbf{RESPONSE:} We've updated the Discussion section to indicate our study is limited by the scope of SDOH explored and acknowledge there are important SDOH, like living environment, access to care, and food security, that are not addressed by our study. \\


\color{default_color} 

-Please talk more about the clinical relevance of this study; how do you perceive clinicians utilizing this information?

\color{comment_color}
\textbf{RESPONSE:} In addition to our previous Discussion section areas which touched on this, we've added the following text:

\begin{quote}
    ``This event-based approach can be used to automatically generate detailed summaries of patient SDOH risk factors. Given that clinicians have limited time to see each patient, automatically populating this information may improve clinician insight into a patient's condition by ensuring they are aware of pertinent information, while reducing the search time necessary to locate it.''
\end{quote}

\color{default_color} 

\section*{Reviewer: 2}

Comments to the Author
This manuscript describes a study to extract SDoH from clinical notes and evaluate the utility of SDoH information from notes by comparing it with structured SDoH information in EHRs. It provides some insights to SDoH in EHR but limited. This reviewer has the following major concerns:

1. A number of papers have developed NLP methods for extracting SDoH from clinical notes, including those from the same authors. It is not clear if mSpERT achieved better performance than other methods, as authors did not include any other STOA methods in the study (no baseline). 

\color{comment_color}
\textbf{RESPONSE:} As described in the response to Reviewer 1, we have compared the performance of mSpERT to the state-of-the-art results in the 2022 n2c2/UW SDOH Challenge.\cite{lybarger2023n2c2} The mSpERT performance would be among the top performing systems in the n2c2/UW SDOH Challenge. We updated the Results to describe the challenge and contextualize the performance of mSpERT. \\



\color{default_color} 

2. SDoH information is sparse in clinical notes and it is distributed differently across different types of notes. It would be interesting if authors can provide more detailed analyses of SDoH information extract from notes by stratifying note type, clinical sub-domain etc.

\color{comment_color}
\textbf{RESPONSE:} Thank you for pointing this out. We have added Tables 6 and 7 to the \textit{Note Distribution} section of the Appendix . Table 6 shows SDOH counts stratified by note type, and Table 7 similarly shows counts by provider specialty. We've also added a brief sentence in Results directing readers to this information. \\

\color{default_color} 

3. Related to \#2, how can we ensure findings about how clinical notes complement structured SDoH data in this study are generalizable for other institutions? Please at least provide some discussion about generalizability of findings at UW.

\color{comment_color}
\textbf{RESPONSE:} We have added the following to the Discussion section:
\begin{quote}
    ``Our study explores the entire patient population at a health system in an urban setting. The study findings may be most generalizable to other urban hospital systems; however, we leave this examination to future work.'' \\
\end{quote}

\color{default_color} 

4. The performance of the NLP system is still suboptimal (some argument types with low performance). How such NLP errors will affect the analysis on the EHR case study?

\color{comment_color}
\textbf{RESPONSE:} We've updated the Results section to be more explicit about the performance of the extracted phenomenon that are most heavily used in the EHR case study. We also updated the Discussion section to acknowledge NLP errors will affect the EHR case study and that the errors disproportionately impact certain SDOH. \\

\color{default_color} 

5. Please provide detailed error analyses on the NLP system.

\color{comment_color}
\textbf{RESPONSE:} We've added a detailed quantitative and qualitative error analysis to the \textit{Error Analysis} section of the Appendix and a brief summary of this error analysis to the Results section. The appendix was used for the more detailed error analysis, due to space constraints. \\

\color{default_color} 

6. Is the overall performance F1 0.86 based on that both event types and arguments are correct?

\color{comment_color}
\textbf{RESPONSE:} The overall performance is micro-averaged across all event types, triggers, and arguments. We've updated the results section to clarify this point. \\

\color{default_color} 

7. In figure 1, why is “not current” not annotated in line 3?

\color{comment_color}
\textbf{RESPONSE:}  In Figure 1, the sentence, ``Prior IV meth \& crack; not current,'' describes past drug use. The \textit{Status Time} argument has subtype label \textit{past}, which can be inferred from the phrases ``Prior'' and ``not current.'' There is ambiguity regarding the annotated span for the \textit{Status Time} argument in this example, as both ``Prior'' and ``not current'' convey status information. Ambiguity in the span annotations for labeled arguments is relatively common. The labeled arguments include subtype labels that capture normalized representation of the span semantics, such that the actual span is less important. The evaluation criteria (see \textit{Scoring Criteria} section of the  Appendix) focuses on the subtype labels and trigger connection for labeled arguments without considering the annotated span.

\color{default_color} 

\bibliography{mybib}
%\bibliographystyle{acl_natbib}




\end{document}
